# Supplementary material for: Spin waves in coupled YIG/Co heterostructures
Source: arXiv:1712.02561 ancillary file (2017-12-07)
Supplement: Supplementary file 1 [file Supplemental_Material_Spin_waves_in_coupled_YIG-Co_heterostructures.pdf]

# Supplemental Material: Spin waves in coupled YIG/Co heterostructures

Stefan Klingler,[1,2,*] Vivek Amin,[3,4] Stephan Geprägs,[1,2] Kathrin Ganzhorn,[1,2] Hannes Maier-Flaig,[1,2] Matthias Althammer,[1,2] Hans Huebl,[1,2,5] Rudolf Gross,[1,2,5] Robert D. McMichael,[3] Mark D. Stiles,[3] Sebastian T.B. Goennenwein,[6,7] and Mathias Weiler[1,2]

[1] *Walther-Meißner-Institut, Bayerische Akademie der Wissenschaften, 85748 Garching, Germany*
[2] *Physik-Department, Technische Universität München, 85748 Garching, Germany*
[3] *Center for Nanoscale Science and Technology, National Institute of Standards and Technology, Gaithersburg, Maryland 20899-6202, USA*
[4] *Institute for Research in Electronics and Applied Physics, University of Maryland, College Park, MD 20742*
[5] *Nanosystems Initiative Munich, 80799 Munich, Germany*
[6] *Institut für Festkörperphysik, Technische Universität Dresden, 01062 Dresden, Germany*
[7] *Center for Transport and Devices of Emergent Materials, Technische Universität Dresden, 01062 Dresden, Germany*

## S1. SAMPLE PREPARATION

The commercially available YIG samples are grown by liquid-phase epitaxy on a (111)-oriented gallium gadolinum garnet substrate to a YIG thickness of $d_2 = 1\ \mu$m. Each sample is cut to lateral dimensions of $(6 \times 5)$ mm$^2$ and is cleaned with Piranha etch and subsequently annealed in oxygen at 500 °C for 40 min [1]. For the first set of samples a thin Co film is deposited onto the YIG film *in-situ* via electron beam evaporation without breaking vacuum. These samples have thicknesses of $d_1 = 35$ nm and $d_1 = 50$ nm (samples YIG/Co(35) and YIG/Co(50), respectively). For a second set of samples a Cu layer with a thickness of $d_\mathrm{s} = 5$ nm is evaporated on the YIG before a Co film with a thickness of $d_1 = 50$ nm is grown on top of it (YIG/Cu(5)/Co(50)). Finally, a control sample is prepared, where a $d_\mathrm{s} = 1.5$ nm thick aluminum (Al) film is sputtered on the YIG with subsequent oxidation. A Co film with a thickness of $d_1 = 50$ nm is subsequently deposited on top of the insulating AlOx via electron beam evaporation (YIG/AlOx(1.5)/Co(50)). All samples are capped with a 2.5 nm thick layer of AlOx to prevent oxidation of the Co layer.

## S2. EXPERIMENTAL SETUP

The dynamic magnetization properties are measured using a vector network analyzer (VNA)-based broadband ferromagnetic resonance setup at room temperature. Fig. S2 shows a sketch of the measurement setup. The YIG/Co samples are placed on a coplanar waveguide (CPW) with the Co side down. The center conductor of the CPW has a width of $w = 300\ \mu$m. The CPW is positioned between the pole shoes of an electromagnet, where magnetic fields of up to 3 T can be applied. The CPW is connected to ports 1 and 2 (P1 and P2, respectively) of the VNA and the complex-valued transmission of a microwave current $j_\mathrm{rf}$ is measured in a frequency range between $f = 1$ GHz and $f = 26.5$ GHz as a function of the applied magnetic field. When the applied frequency $f$ matches the resonance condition for a given field $\boldsymbol{H}$, microwave power is absorbed, which results in a precession of the samples magnetization. As the transmission signal of the CPW is strongly frequency dependent, we do not show the raw frequency spectra in the main text, but the field-derivative of $S_{21}$ as shown in Ref. [2] and S3.

## S3. DERIVATIVE DIVIDE - EXPERIMENT AND SIMULATIONS

The measured transmission of the vector network analyzer is given by:

$$S_{21}(H) = \Delta S_{21}(H) S_{21}^0 + S_{21}^0. \tag{S3.1}$$

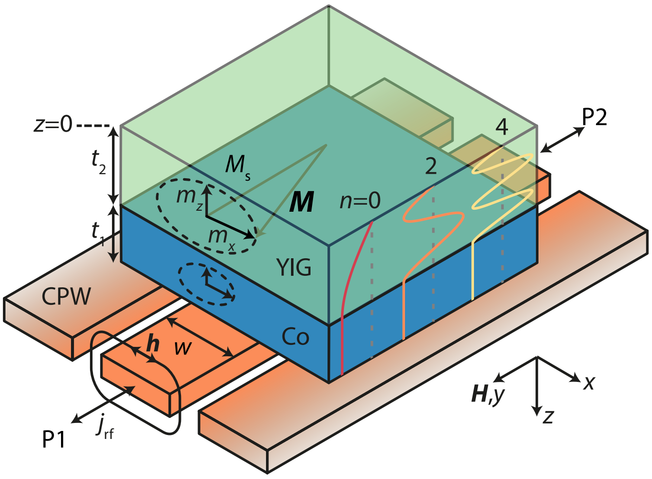


FIG. S2. Sketch of the measurement setup. The YIG/Co samples are positioned with the Co-side down onto the center conductor of the CPW.

* stefan.klingler@wmi.badw.de

Here, $S_{21}^0$ is the field-independent background transmission. Note that a perfect background transmission is achieved for $S_{21}^0 = 1$. The measurement signal is given by [3]:

$$\Delta S_{21}(H) = -i\omega \frac{L_0(H)}{2Z_0}, \qquad \text{(S3.2)}$$

where $L_0$ is the inductance of the sample and $Z_0 = 50\ \Omega$ is the microwave circuit impedance. The sample inductance is given by [4]:

$$L_0(H) = \frac{\mu_0 l d_{\mathrm{tot}}}{4w}\chi(H), \qquad \text{(S3.3)}$$

where $l = 5$ mm is the length of the sample, $d_{\mathrm{tot}} \approx 1\ \mu$m is the total thickness of the sample, $w = 300\ \mu$m is the width of the center conductor, and $\chi(H)$ is the dynamic magnetic susceptibility.

The background-corrected field derivative of our measurement signal is now given by [2]:

$$\partial_{\mathrm{D}} S_{21}/\partial H = \frac{1}{S_{21}(H)} \frac{S_{21}(H+\delta H) - S_{21}(H-\delta H)}{\delta H}, \qquad \text{(S3.4)}$$

where $\delta H$ is a constant field step in our measurement of about 0.5 mT. Note that the differential quotient is rescaled by the central value $S_{21}(H)$ which eliminates background drift.

We simulate $\chi = \chi_{1,xx}$, from which we calculate $\Delta S_{21}$ with Eq. (S3.2), where $\chi_{1,xx}$ creates the $x$-component of the dynamic magnetization in the limit of $w > d_{\mathrm{tot}}$. To compare the simulation results to experimental data, we use Eq. (S3.1) with $S_{21}^0 = 1$ and then calculate $\partial_{\mathrm{D}} S_{21}/\partial H$ from Eq. (S3.3) which yields:

$$\begin{aligned}\partial_{\mathrm{D}} S_{21}/\partial H &= \frac{\Delta S_{21}(H+\delta H) - \Delta S_{21}(H-\delta H)}{(\Delta S_{21}(H)+1)\delta H} \\ &= \frac{d_{\mathrm{tot}} l \mu_0 \omega (\chi_{1,xx}(\delta H + H) - \chi_{1,xx}(H-\delta H))}{\delta H (d_{\mathrm{tot}} l \mu_0 \omega \chi_{1,xx}(H) + 8 i w Z_0)}.\end{aligned} \qquad \text{(S3.5)}$$

The susceptibility element $\chi_{1,xx}$ is derived in S9.

## S4. DETERMINATION OF MATERIAL PARAMETERS

Fig. S4 (a) shows the extracted resonance fields as a function of the frequency for the YIG/Co(35) sample using a fit of up to five superimposed Lorentzian resonances. The inset shows a magnification of the field and frequency range marked with the dashed box, and we observe multiple avoided crossings. The frequency splitting $g_{\mathrm{eff}}$ is determined using a fit of a coupled harmonic oscillator model to the avoided crossings, as shown in [11].

To obtain the material parameters of the Co layer, we fit the pure Co FMR line which we get by deleting all data points of avoided crossings and YIG PSSWs from the data set, as shown in Fig. S4 (b). For the fit we use the in-plane Kittel equation,

$$f_i = \frac{\mu_0 \gamma_i}{2\pi}\sqrt{(H + H_{\mathrm{ex},i})(H + H_{\mathrm{ex},i} + M_{\mathrm{s},i})} \qquad \text{(S4.1)}$$

which yields $\gamma_1/2\pi = 28.7(1)$ GHz/T and $\mu_0 M_{\mathrm{s},1} = 1.91(2)$ T, where the number in brackets denotes the error of the last digit. The fit is shown as a black line.

To obtain the material parameters of the YIG film, we fit the pure YIG PSSWs, as shown in Fig. S4 (c). We keep $\mu_0 M_{\mathrm{s},2} = 0.18$ T constant, as we otherwise get a mutual dependence of $M_{\mathrm{s},2}$ and $H_{\mathrm{ex},2}$ during the fit [5]. A global fit, where $\gamma_1$ in Eq. (S4.1) is a shared fit parameter and $H_{\mathrm{ex},i}$ is fitted for each PSSW individually, yields $\gamma_2/2\pi = 27.07(1)$ GHz/T. The fits are shown as black lines.

The values of the YIG and the Co film agree very well with the literature values [5–8] and they are thus taken to be constant throughout for the data analysis.

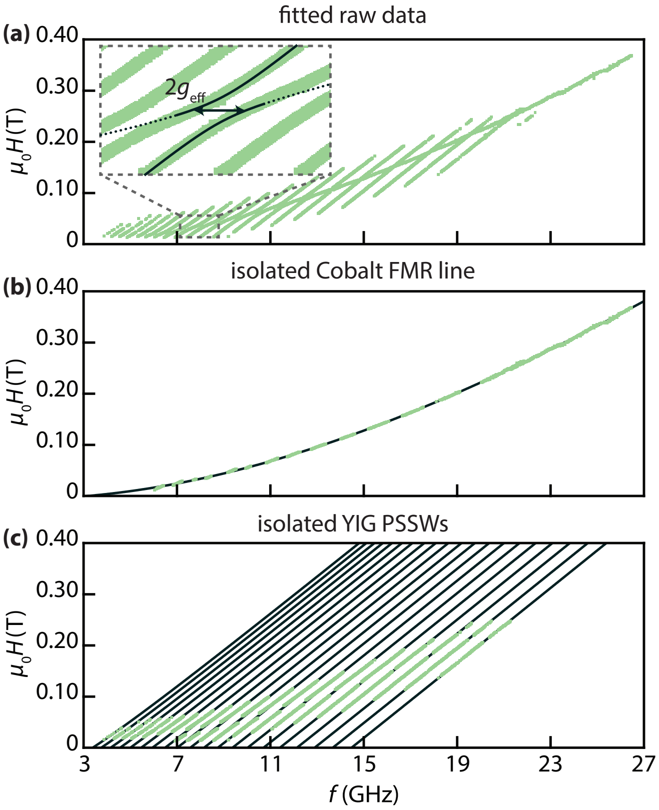


FIG. S4. (a) Fitted raw data resonance fields and frequencies of the YIG/Co(35) sample. (b) Isolated Co FMR line. (c) Isolated YIG PSSWs.

## S5. DETERMINATION OF THE EXCHANGE STIFFNESS

In Fig. S5 (a), an example frequency spectrum is shown for the YIG/Co(50) sample for a fixed field of $\mu_0 H =$

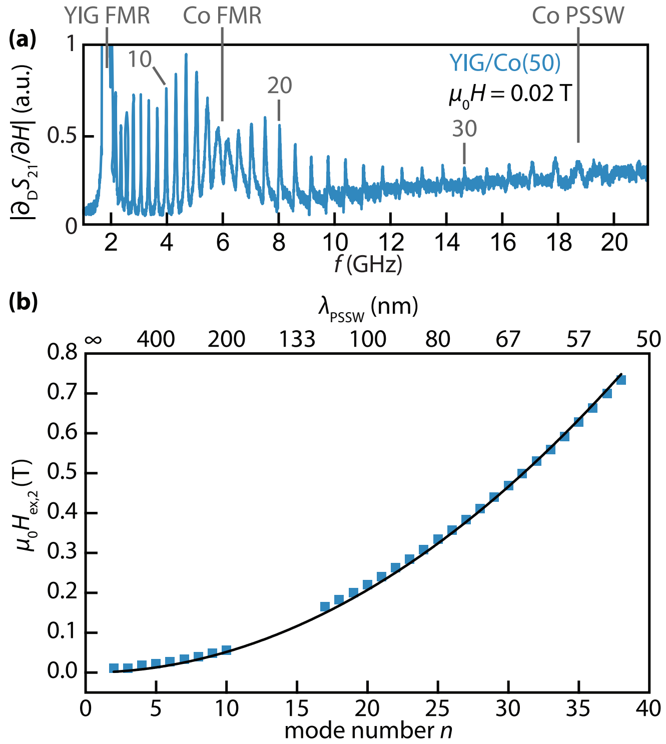


FIG. S5. (a) Example frequency spectrum of the YIG/Co(50) sample at $\mu_0 H = 0.02$ T. (b) The extracted exchange fields of the YIG/Co(50) sample are plotted as a function of the PSSW mode number $n$.

0.02 T. Plotted is $|\partial_D S_{21}/\partial H|$ versus applied microwave frequency, and the plot corresponds to a cut along the $x$-axis in Fig. 1 (a). The peak in $|\partial_D S_{21}/\partial H|$ at 2 GHz is attributed to the YIG FMR frequency. At about 6 GHz we find a broad excitation of the Co FMR. Furthermore, we resolve about 40 YIG PSSW resonances. Some of the YIG PSSWs are labeled to guide the reader. In comparison to Ref. [5] we find a drastically increased sensitivity for the YIG PSSWs. Furthermore, all PSSWs are equally visible, not only the modes with an odd mode number. This is expected for driving fields which are strongly inhomogeneous, but cannot be explained with the width of the used center conductor, which is much larger than the YIG film thickness.

From the extracted resonance fields of each YIG mode, we are able to determine the exchange fields, see S4. For this we assume a fixed saturation magnetization of $\mu_0 M_{s,2} = 0.18$ T [8]. We then use the method proposed in Ref. [5] to determine the exchange stiffness $D_s$. In Fig. S5 (b), the extracted exchange fields are shown as a function of the mode number $n$. We see a quadratic curvature (black) of the exchange field, which is fitted using:

$$\mu_0 H_{ex,2} = D_{s,2} \left( \frac{n\pi}{d_2} \right)^2 . \tag{S5.1}$$

From the fit a value of $D_{s,2} = 5.25(2) \times 10^{-17}$ T m$^2$ is obtained, which is in very good agreement with previously reported values [5, 9]. Using the relation $A_i = D_{s,i} M_{s,i}/2$ we yield $A_2 = A = 3.76$ pJ/m. Furthermore, the quadratic increase of the exchange fields with the mode number $n$ and the extracted value of $D_{s,i}$ confirm our assumption that we indeed observe standing spin-wave modes in the YIG film. Note that we only expect minor interfacial corrections to for $H_{ex,2}(k)$ for mixed boundary conditions.[1]

## S6. TRANSMISSION SPECTRA YIG/Co(35)

Fig. S6 (a) shows the background-corrected field derivative of the transmission spectra for the YIG/Co(35) heterostructure. Again we observe the high and the low frequency mode which correspond to the Co and YIG FMR lines, respectively, together with the exchange mode. The YIG PSSWs form avoided crossings with the Co FMR line as shown in magnification (inset). The frequency splitting has about the same size as found from the YIG/Co(50) heterostructure and be simulated with similar parameters. Here, we show that these parameters are not unique. Fig. S6 (b) shows the simulation for the YIG/Co(35) heterostructure using a negative field-like torque and a ferromagnetic coupling, in contrast to the simulations in the main text. This parameter set also models the avoided crossings. However, the intensity asymmetry of the avoided crossings is only reproduced with the ferromagnetic coupling if the field-like torque is negative, as shown in Fig. S6 (b). For more details, see S10.

## S7. CO LINEWIDTH EVOLUTION OF THE YIG/AlOx(1.5)/Co(50) SAMPLE

In this section we analyze the linewidth evolution of the YIG/AlOx/Co(50) sample and compare it to the YIG/Co(50) sample to show that the magnetizations are uncoupled. Even a weak coupling of the YIG and the Co magnetizations should be visible in the linewidth evaluations of the subsystems [10, 11], as the coupling opens additional relaxation channels, which is reflected in the lifetimes of the spin-wave resonances. In Fig. S7 the linewidth evolution of the YIG/Co(50) sample is shown as a function of the excitation frequency (blue symbols). We find for $f < 14$ GHz a strong modulation of the linewidth. This modulation goes along with the observation of avoided crossings in Fig. 1 (a). However, in Fig. S7 also the Co linewidth from the YIG/AlOx(1.5)/Co(50) sample (orange symbols) is shown as a function of the

[1] If we assume total pinning of the YIG magnetization at both interfaces, we obtain a small deviation of 4 % to the extracted value of $D_{s,2}$.

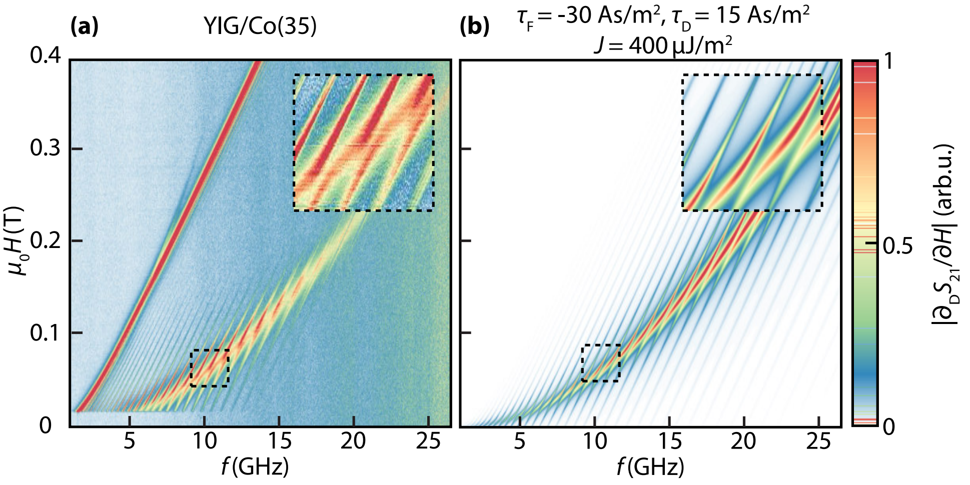


FIG. S6. (a) Transmission spectra of the YIG/Co(35). (b) Simulation of the of the YIG/Co(35) sample using the inverted field-like and exchange torques as in the main text for the YIG/Co(50) sample.

excitation frequency. For small frequencies we see a fast increase of the linewidth which flattens out above $f = 10$ GHz. The shape of this linewidth evolution can be understood with Gilbert damping and two-magnon scattering processes, which are expected for an in-plane measurement geometry [12–18]. There are no additional features that indicate any coupling of the YIG and the Co in the YIG/AlOx(1.5)/Co(50) heterostructure. Hence, we can rule out dynamic stray fields as the origin of the coupling. From the YIG/AlOx(1.5)/Co(50) sample we extract a Gilbert damping parameter $\alpha_1$ of the Co layer

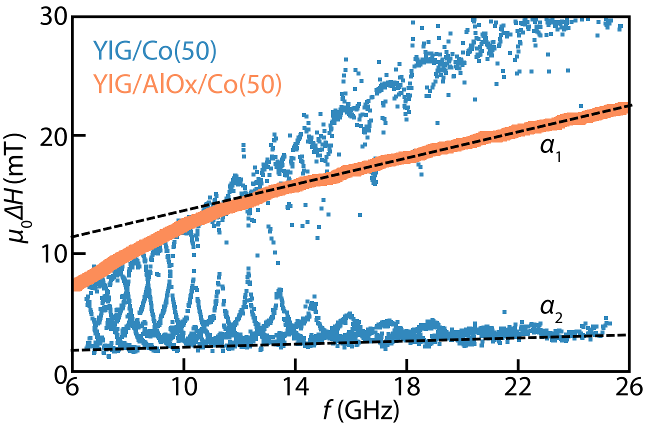


FIG. S7. The linewidth evolution of the YIG/Co(50) and YIG/AlOx(1.5)/Co(50) samples is shown as a function of the excitation frequency. The linewidth of the YIG/AlOx(1.5)/Co(50) sample increases monotonically (orange symbols), without any modulation. The blue symbols show the linewidths of the YIG/Co(50) sample which shows characteristic modulation for every coupled PSSW.

using the Gilbert damping equation [19]:

$$\mu_0 \Delta H_i = \mu_0 \Delta H_{0,i} + \frac{4\pi\alpha_i}{\gamma_i} f, \tag{S7.1}$$

where $\Delta H_1$ is the Co linewidth and $\Delta H_{0,1}$ the inhomogeneous line broadening of the Co film. The fit is shown as the black dashed line in Fig. S7 and we obtain an intrinsic Gilbert damping of $\alpha_1 = 0.0077 \pm 0.0001$ and $\mu_0 \Delta H_{0,1} = (8 \pm 1)$ mT. Hence, approximately half of the linewidth of the Co resonance is due to the frequency independent inhomogeneous line broadening. The YIG damping can be estimated in a similar way from the coupled YIG/Co(50) sample to be $\alpha_2 = (7.2 \pm 0.3) \times 10^{-4}$, which is in good agreement with previous reports [6] .

## S8. DYNAMIC SPIN TORQUE IN A FM$_1$|NM|FM$_2$ HETEROSTRUCTURE

We write the following equations in terms of the magnetization density and magnetization current. We assume a large applied field in the $y$-direction which aligns the magnetization. The film lies in the $x-y$-plane, whereas the film normal points along the $z$-direction (S2). We also assume that the transverse magnetizations are small and decouple from the charge and longitudinal magnetization. It is convenient to write the equations of motion in terms of complex numbers made up of the transverse components. Thus we express the vector $\boldsymbol{f} = (f_x, 1, f_z)$ as follow:

$$\mathrm{f}_\perp = f_z + i f_x \leftrightarrow \begin{pmatrix} \mathrm{Re}\,[\mathrm{f}_\perp] \\ \mathrm{Im}\,[\mathrm{f}_\perp] \end{pmatrix} = \begin{pmatrix} f_z \\ f_x \end{pmatrix}. \tag{S8.1}$$

In this notation, the cross product operation $(0,1,0) \times (f_x, 1, f_z) = (f_z, 0, -f_x)$ can be represented as multiplica-

tion with the imaginary unit $i$

$$(\hat{\boldsymbol{y}} \times \boldsymbol{f})_\perp \to -f_x + i f_z = i(f_z + i f_x) = i\mathsf{f}_\perp. \quad \text{(S8.2)}$$

In the following we drop the subscript $\perp$ from the complex representation of vectors (without serifs and upright) for simplicity.

We consider a ferromagnet|normal metal|ferromagnet ($\mathrm{FM}_1$|NM|$\mathrm{FM}_2$) heterostructure, where the spacer layer $d_\mathrm{s}$ is thick compared to its mean free path but thin compared to the spin diffusion length. The first assumption allows us to use the drift-diffusion approach to treat the transport. The second assumption allows us to neglect spin-flip scattering in the spacer layer, in which case the spin accumulation varies linearly across the spacer layer. In this case the transverse spin current density $\mathsf{j} = 2e\mathsf{Q}/\hbar$ (in units of V, the traditional spin current density is given by $\mathsf{Q}$) in the spacer layer can be written as follows:

$$\begin{aligned} \mathsf{j}(z) &= -D\nabla\mu(z) \\ &= -D\nabla(\mu_0 + \mu' z) \\ &= -D\mu'. \end{aligned} \quad \text{(S8.3)}$$

Here, $\mu(z) = (\mu_\uparrow - \mu_\downarrow)/e$ is the spin accumulation in the spacer (units of V), also written as a complex number; and $D = \sigma_\mathrm{NM}$ (units of $1/\Omega\,\mathrm{m}$), where $\sigma_\mathrm{NM}$ is the bulk conductivity of the normal metal. Note that we work with spin accumulation rather than spin density; this gives the constant $D$ units of $1/\Omega\,\mathrm{m}$ rather than $\mathrm{m}^2/\mathrm{s}$. In the second line we have used a linear expansion of the spin accumulation, where $\mu' = \partial\mu/\partial z$. We find that the spatially-constant spin current density is proportional to the gradient of the spin accumulation.

We assume the spacer layer has length $d_\mathrm{s}$, running from $z = -d_\mathrm{s}/2$ to $z = d_\mathrm{s}/2$ (Without loss of generality, we have shifted here the origin of the coordinate system to the center of the spacer layer, in contrast to the other sections). For the boundary conditions at the first interface ($z = -d_\mathrm{s}/2$), we have

$$\begin{aligned} -D\mu' &= \mathsf{j}(-d_\mathrm{s}/2) \\ &= -\mathsf{G}_1\mu + \frac{\hbar}{4\pi e}\mathsf{G}_1 i\dot{\mathsf{m}}_1 \\ &= -\mathsf{G}_1(\mu_0 - \mu' d_\mathrm{s}/2) + \frac{\hbar}{4\pi e}\mathsf{G}_1 i\dot{\mathsf{m}}_1. \end{aligned} \quad \text{(S8.4)}$$

Here, $\mathsf{G}_1$ is the complex spin mixing conductance of the first interface (units of $1/\Omega\,\mathrm{m}^2$). The top line gives the spin current in the spacer layer and the second line is the boundary condition from magnetoelectronic circuit theory with the second term the pumped spin current. In the second line, we have used $\boldsymbol{M}_1 \times \dot{\boldsymbol{M}}_1 \approx \hat{\boldsymbol{y}} \times \dot{\boldsymbol{M}}_1 \to i\dot{\mathsf{m}}_1$ The boundary condition at the other interface ($z = d_\mathrm{s}/2$) is the same except that the signs change because the direction of the interface normal changes:

$$\begin{aligned} \mathsf{j}(d_\mathrm{s}/2) &= -D\mu' \\ &= \mathsf{G}_2(\mu_0 + \mu' d_\mathrm{s}/2) - \frac{\hbar}{4\pi e}\mathsf{G}_2 i\dot{\mathsf{m}}_2. \end{aligned} \quad \text{(S8.5)}$$

The boundary conditions then give us four equations in four unknowns ($\mu_{0z}$, $\mu_{0x}$ $\mu'_z$, $\mu'_x$), or two complex equations Eq. (S8.4) and Eq. (S8.5) in two complex unknowns ($\mu_0$, $\mu'$). We find

$$\begin{aligned} \mu_0 &= \frac{i\hbar}{4\pi e}\frac{2D(\mathsf{G}_1\dot{\mathsf{m}}_1 + \mathsf{G}_2\dot{\mathsf{m}}_2) + d_\mathrm{s}\mathsf{G}_1\mathsf{G}_2(\dot{\mathsf{m}}_1 + \dot{\mathsf{m}}_2)}{2(D(\mathsf{G}_1 + \mathsf{G}_2) + d_\mathrm{s}\mathsf{G}_1\mathsf{G}_2)}, \\ \mu' &= -\frac{i\mathsf{G}_1\mathsf{G}_2\hbar(\dot{\mathsf{m}}_1 - \dot{\mathsf{m}}_2)}{4\pi e(D(\mathsf{G}_1 + \mathsf{G}_2) + d_\mathrm{s}\mathsf{G}_1\mathsf{G}_2)}, \end{aligned} \quad \text{(S8.6)}$$

from which we can derive the spin current

$$\mathsf{j}(-d_\mathrm{s}/2) = -i\frac{\hbar}{4\pi e}\mathsf{G}(\dot{\mathsf{m}}_1 - \dot{\mathsf{m}}_2). \quad \text{(S8.7)}$$

Here we have defined an effective mixing conductance that describes the coupled system:

$$\mathsf{G} = \frac{\mathsf{G}_1\mathsf{G}_2}{\mathsf{G}_1 + \mathsf{G}_2 + \mathsf{G}_1\mathsf{G}_2 d_\mathrm{s}/D} \approx \frac{\mathsf{G}_1\mathsf{G}_2}{\mathsf{G}_1 + \mathsf{G}_2}, \quad \text{(S8.8)}$$

where we have used the small $d_\mathrm{s}$ limit in the second step in the denominator, as the conductance of a thin Cu layer is much greater than either mixing conductance (the Cu interlayer is much thinner than the spin-diffusion length of Cu). Note that in this limit the amplitudes of the spin currents persist, when we remove the Cu layer. However, in this case the exchange coupling starts to play a major role.

In the absence of spin-orbit coupling, the spin torque exerted on some region equals the difference between the spin currents at the boundaries of that region. The transverse spin current just inside the ferromagnets vanish due to dephasing, i.e., $\mathsf{j}(-d_\mathrm{s}/2 - \epsilon) = 0$ and $\mathsf{j}(d_\mathrm{s}/2 + \epsilon) = 0$. So, the spin torque, $\tau_1$, also a complex number representing the two transverse components, at the first interface is given by

$$\begin{aligned} \mathsf{\tau}_1 =& \Delta\mathsf{j} \\ =& \mathsf{j}(-d_\mathrm{s}/2 + \epsilon) - \mathsf{j}(-d_\mathrm{s}/2 - \epsilon) \\ =& \mathsf{j}(-d_\mathrm{s}/2 + \epsilon), \end{aligned} \quad \text{(S8.9)}$$

where the $x$ and $z$ components are extracted according to the prescription given above:

$$\tau_{1,z} = \mathrm{Re}[\mathsf{j}], \quad \text{(S8.10)}$$
$$\tau_{1,x} = \mathrm{Im}[\mathsf{j}]. \quad \text{(S8.11)}$$

Since the interface normal flips between the two interfaces, the torques on the two magnetizations are equal and opposite (i.e., $\tau_1 = -\tau_2$). Note that here the torques have the same units as the normalized spin current density.

We now want to show how the spin torques are included in the Landau-Lifshitz-Gilbert equation. Assuming a time dependence of the magnetization

$$\mathsf{m}_i = (m_{i,z}, m_{i,x})\exp(-i\omega t), \quad \text{(S8.12)}$$

the spin torque on the first ferromagnet is given by

$$\begin{aligned}\boldsymbol{\tau}_1 =& -i\frac{\hbar}{4\pi e}\mathsf{G}(-i\omega)(\mathsf{m}_1-\mathsf{m}_2)\\ =& -\omega\frac{\hbar}{4\pi e}\mathsf{G}(\mathsf{m}_1-\mathsf{m}_2),\end{aligned} \tag{S8.13}$$

and similarly the spin torque on the second ferromagnet is given by

$$\boldsymbol{\tau}_2 = \omega\frac{\hbar}{4\pi e}\mathsf{G}(\mathsf{m}_1-\mathsf{m}_2) = -\boldsymbol{\tau}_1. \tag{S8.14}$$

Hence, the torques depend on the real and imaginary parts of the effective mixing conductance $\mathsf{G}$. Unfortunately, extracting the mixing conductances for each interface is impossible unless one mixing conductance is already known.

In the following we show how the torques can be introduced to the LLG. After a complex multiplication we obtain from Eq. (S8.13) and Eq. (S8.14):

$$\begin{aligned}\tau_{1,z} = \mathrm{Re}[\boldsymbol{\tau}_1] &= -\omega\frac{\hbar}{4\pi e}\Big(\mathrm{Re}[\mathsf{G}]\mathrm{Re}[\mathsf{m}_1-\mathsf{m}_2]-\mathrm{Im}[\mathsf{G}]\mathrm{Im}[\mathsf{m}_1-\mathsf{m}_2]\Big)\\ &= -\omega\Big(\tau_\mathrm{D}(m_{1,z}-m_{2,z})-\tau_\mathrm{F}(m_{1,x}-m_{2,x})\Big)\end{aligned} \tag{S8.15}$$

$$\begin{aligned}\tau_{1,x} = \mathrm{Im}[\boldsymbol{\tau}_1] &= -\omega\frac{\hbar}{4\pi e}\Big(\mathrm{Im}[\mathsf{G}]\mathrm{Re}[\mathsf{m}_1-\mathsf{m}_2]+\mathrm{Re}[\mathsf{G}]\mathrm{Im}[\mathsf{m}_1-\mathsf{m}_2]\Big)\\ &= -\omega\Big(\tau_\mathrm{F}(m_{1,z}-m_{2,z})+\tau_\mathrm{D}(m_{1,x}-m_{2,x})\Big),\end{aligned} \tag{S8.16}$$

and analogously

$$\tau_{2,z} = \mathrm{Re}[\boldsymbol{\tau}_2] = \omega\Big(\tau_\mathrm{D}(m_{1,z}-m_{2,z})-\tau_\mathrm{F}(m_{1,x}-m_{2,x})\Big) \tag{S8.17}$$

$$\tau_{2,x} = \mathrm{Im}[\boldsymbol{\tau}_2] = \omega\Big(\tau_\mathrm{F}(m_{1,z}-m_{2,z})+\tau_\mathrm{D}(m_{1,x}-m_{2,x})\Big), \tag{S8.18}$$

where we have defined the torque strengths (units of $\mathrm{A\,s/m^2}$) as

$$\tau_\mathrm{D} = \frac{\hbar}{4\pi e}\mathrm{Re}[\mathsf{G}], \tag{S8.19}$$

$$\tau_\mathrm{F} = \frac{\hbar}{4\pi e}\mathrm{Im}[\mathsf{G}]. \tag{S8.20}$$

Note that multiplying a torque strength ($\tau_{\mathrm{D/F}}$) by the time derivative of a magnetization unit vector gives a torque in units of $\mathrm{A/m^2}$. The torque on the second interface ($\boldsymbol{\tau}_2$) is obtained in a similar manner. The expressions for both torques can be written in matrix notation as follows:

$$\begin{pmatrix}\tau_{1,z}\\ \tau_{1,x}\\ \tau_{2,z}\\ \tau_{2,x}\end{pmatrix} = -\omega\begin{pmatrix}\tau_\mathrm{D} & -\tau_\mathrm{F} & -\tau_\mathrm{D} & \tau_\mathrm{F}\\ \tau_\mathrm{F} & \tau_\mathrm{D} & -\tau_\mathrm{F} & -\tau_\mathrm{D}\\ -\tau_\mathrm{D} & \tau_\mathrm{F} & \tau_\mathrm{D} & -\tau_\mathrm{F}\\ -\tau_\mathrm{F} & -\tau_\mathrm{D} & \tau_\mathrm{F} & \tau_\mathrm{D}\end{pmatrix}\begin{pmatrix}m_{1,z}\\ m_{1,x}\\ m_{2,z}\\ m_{2,x}\end{pmatrix}. \tag{S8.21}$$

Here the torques still have units of charge current density. To convert the torque strengths into a form consistent with the LLG equations, they must be multiplied by

$$-\frac{\hbar\gamma_i}{ed_iM_{s,i}}, \tag{S8.22}$$

where $i \in [1,2]$ denotes the material, $\gamma_i$ is the gyromagnetic ratio, $M_{s,i}$ is the saturation magnetization, and $d_i$ is the magnetic film thickness.

## S9. THE INTERFACIAL SPIN-TORQUE MODEL

Here, we derive a model for the dynamic mode coupling at the YIG/Co interface. For this we use a macrospin approximation for the Co magnetization ($\boldsymbol{M}_1$), as we only consider the first cobalt mode. However, we assume that the unit vector of YIG magnetization direction ($\boldsymbol{M}_2(z)$) varies spatially. In section S8, a real-valued two-vector was represented as a single complex number. Here, we adopt a notation of using lower case bold letters to indicate the transverse components. In addition, to capture the phases of the precessing moments, we allow these vectors to be complex with the understanding that the real part should be taken of a results to get physical quantities. As in the main text, upper case bold characters indicate three-dimensional vectors.

In the limit of small transverse magnetization, the energy of the coupled heterostructure is given by:

$$\begin{aligned} E = &\int_0^{d_2} dz \left[ A\left(\partial_z \boldsymbol{m}_2\right)^2 + \frac{\mu_0 H M_{\mathrm{s},2}}{2} \boldsymbol{m}_2 \cdot \boldsymbol{m}_2 + \frac{\mu_0 M_{\mathrm{s},2}^2}{2} m_{2,z}^2 \right] \\ &+ \frac{\mu_0 H M_{\mathrm{s},1} d_1}{2} \boldsymbol{m}_1 \cdot \boldsymbol{m}_1 + \frac{\mu_0 M_{\mathrm{s},1}^2 d_1}{2} m_{1,z}^2 + J(\boldsymbol{m}_1 - \boldsymbol{m}_2(d_2))^2. \end{aligned} \tag{S9.1}$$

Here, the integrand describes the energy contribution of the YIG film. All variable definitions are given in the main text.

We obtain the effective field of the Co by using the magnetic energy which is normalized on the Co thickness and saturation magnetization: $H_{\mathrm{eff},1} = -\nabla E/(M_{\mathrm{s},1} d_1)$. We can hence write down the linearized Landau-Lifshitz-Gilbert equation for the Co film:

$$\begin{aligned} \dot{\boldsymbol{m}}_1 = &-\gamma_1 \hat{\boldsymbol{y}} \times \left[ -\mu_0 H \boldsymbol{m}_1 - \frac{\alpha_1}{\gamma_1} \dot{\boldsymbol{m}}_1 - \mu_0 M_{s,1} M_{1,z} \hat{\boldsymbol{z}} - \frac{J}{d_1 M_{s,1}} (\boldsymbol{m}_1 - \boldsymbol{m}_2(d_2)) + \mu_0 \boldsymbol{h} \right] \\ &- \frac{\hbar \gamma_1}{e d_1 M_{s,1}} \left[ (\tau_{\mathrm{F}} - \tau_{\mathrm{D}} \hat{\boldsymbol{y}} \times)(\dot{\boldsymbol{m}}_1 - \dot{\boldsymbol{m}}_2(d_2)) \right]. \end{aligned} \tag{S9.2}$$

Here we have used that the static magnetization lies along in the film plane, parallel to the external magnetic field along the $y$-direction. Analogously, we derive the equation of motion for the YIG away from the interface:

$$\dot{\boldsymbol{m}}_2 = -\gamma_2 \hat{\boldsymbol{y}} \times \left[ -\mu_0 H \boldsymbol{m}_2 - \frac{\alpha_2}{\gamma_2} \dot{\boldsymbol{m}}_2 - \mu_0 M_{\mathrm{s},2} m_{2,z} \hat{\boldsymbol{z}} + \frac{2A}{M_{\mathrm{s},2}} \partial_z^2 \boldsymbol{m}_2 + \mu_0 \boldsymbol{h} \right], \tag{S9.3}$$

where the definitions of the variables is analogous to the Co variables, except of the index 2 instead of 1. The coupling terms will be treated as a boundary condition.

### A. Determination of the Eigenvectors

We know that the magnetization in the YIG is a superposition of the eigenmodes in the undisturbed film. In order to determine those, we start by rewriting Eq. (S9.3) in a notation of the transverse magnetization. By using the ansatz for the transverse magnetization components

$$\boldsymbol{m}_2 = \exp(ikz)\exp(-i\omega t) \begin{pmatrix} m_{2,z} \\ m_{2,x} \end{pmatrix}, \tag{S9.4}$$

we obtain a system of equations including the YIG susceptibility $\tilde{\boldsymbol{\chi}}_2^{-1}$, which describes the response of the transverse YIG magnetization perpendicular to external magnetic fields:

$$0 = \underbrace{\begin{pmatrix} -i\omega & \gamma_2\left(\frac{2Ak^2}{M_{\mathrm{s},2}} + \mu_0 H\right) - i\alpha_2\omega \\ \gamma_2\left(-\frac{2Ak^2}{M_{\mathrm{s},2}} - \mu_0 H - \mu_0 M_{\mathrm{s},2}\right) + i\alpha_2\omega & -i\omega \end{pmatrix}}_{\tilde{\boldsymbol{\chi}}_2^{-1}} \begin{pmatrix} m_{2,z} \\ m_{2,x} \end{pmatrix}. \tag{S9.5}$$

The system of equations is solved for $\det \tilde{\boldsymbol{\chi}}_2^{-1} = 0$ by the wavevectors:

$$k = \frac{1}{2}\sqrt{\frac{M_{\mathrm{s},2}\left(2i\alpha_2\omega - \gamma_2\mu_0(2H + M_{\mathrm{s},2}) + \sqrt{\gamma_2^2\mu_0^2 M_{\mathrm{s},2}^2 + 4\omega^2}\right)}{A\gamma_2}}, \tag{S9.6}$$

$$k = i\kappa = \frac{1}{2}\sqrt{-\frac{M_{\mathrm{s},2}\left(-2i\alpha_2\omega + \gamma_2\mu_0(2H + M_{\mathrm{s},2}) + \sqrt{\gamma_2^2\mu_0^2 M_{\mathrm{s},2}^2 + 4\omega^2}\right)}{A\gamma_2}}. \tag{S9.7}$$

The wavevector $k$ describes an harmonic oscillation of the magnetization along the $z$-direction. The wavevector $\kappa$ on the other side describes an evanescent behavior of the YIG magnetization, with a decay length in the order of 10 nm.

We now use the obtained wavevectors in Eq. (S9.5) in order to derive the eigenvectors of the YIG magnetization. For the wavevectors $k$ and $\kappa$ we obtain

$$k: \ 0 = \begin{pmatrix} -i\omega & \frac{1}{2}\left(-M_{\mathrm{s},2}\gamma_2\mu_0 + \sqrt{M_{\mathrm{s},2}^2\gamma_2^2\mu_0^2 + 4\omega^2}\right) \\ \frac{1}{2}\left(-M_{\mathrm{s},2}\gamma_2\mu_0 - \sqrt{M_{\mathrm{s},2}^2\gamma_2^2\mu_0^2 + 4\omega^2}\right) & -i\omega \end{pmatrix} \begin{pmatrix} m_{2,z} \\ m_{2,x} \end{pmatrix}, \tag{S9.8}$$

$$\kappa: \ 0 = \begin{pmatrix} -i\omega & \frac{1}{2}\left(-M_{\mathrm{s},2}\gamma_2\mu_0 - \sqrt{M_{\mathrm{s},2}^2\gamma_2^2\mu_0^2 + 4\omega^2}\right) \\ \frac{1}{2}\left(-M_{\mathrm{s},2}\gamma_2\mu_0 + \sqrt{M_{\mathrm{s},2}^2\gamma_2^2\mu_0^2 + 4\omega^2}\right) & -i\omega \end{pmatrix} \begin{pmatrix} m_{2,z} \\ m_{2,x} \end{pmatrix}. \tag{S9.9}$$

We now take the zero eigenvalue of both systems, as this refers to our resonance condition $\det \tilde{\chi}_2^{-1} = 0$. We find

$$k: \ \boldsymbol{m}_{2+} = \begin{pmatrix} \frac{i\left(-\sqrt{\gamma_2^2\mu_0^2 M_{\mathrm{s},2}^2 + 4\omega^2} + \gamma_2\mu_0 M_{\mathrm{s},2}\right)}{2\omega} \\ 1 \end{pmatrix}, \tag{S9.10}$$

$$\kappa: \ \boldsymbol{m}_{2-} = \begin{pmatrix} \frac{i\left(\sqrt{\gamma_2^2\mu_0^2 M_{\mathrm{s},2}^2 + 4\omega^2} + \gamma_2\mu_0 M_{\mathrm{s},2}\right)}{2\omega} \\ 1 \end{pmatrix}. \tag{S9.11}$$

### B. Setup of the Boundary Conditions

We model the YIG/Co interface as an infinitesimally thin surface layer. While the magnetization is not pinned at the interface, the infinitesimally thin layer has no volume and hence no angular momentum. As a consequence, the total torque acting at the interface has to vanish:

$$\begin{aligned} 0 =& 2A\hat{\boldsymbol{y}} \times \partial_z \boldsymbol{m}_2(z)|_{z=d_2} - J\hat{\boldsymbol{y}} \times (\boldsymbol{m}_1 - \boldsymbol{m}_2(d_2)) \\ &+ (\hbar/e)(\tau_{\mathrm{F}} - \tau_{\mathrm{D}}\hat{\boldsymbol{y}}\times)\,(\dot{\boldsymbol{m}}_1 - \dot{\boldsymbol{m}}_2(d_2))\,. \end{aligned} \tag{S9.12}$$

On the YIG/substrate interface we also set the torques to be zero:

$$0 = 2A\hat{\boldsymbol{y}} \times \partial_z \boldsymbol{m}_2(z)|_{z=0} \tag{S9.13}$$

### C. Solution of the Problem

The ansatz of the dynamic YIG magnetization $\boldsymbol{m}_2$ and the dynamic Co magnetization $\boldsymbol{m}_1$ are

$$\begin{aligned} \boldsymbol{m}_2 =& + c_-\boldsymbol{m}_{2-}\exp(-i\omega t)\cos(\kappa z) \\ &+ c_+\boldsymbol{m}_{2+}\exp(-i\omega t)\cos(kz), \end{aligned} \tag{S9.14}$$

and

$$\boldsymbol{m}_1 = \begin{pmatrix} m_{z,1} \\ m_{x,1} \end{pmatrix}\exp(-i\omega t). \tag{S9.15}$$

In a first step we rewrite the boundary condition Eq. (S9.12):

$$\begin{aligned} 0 =& + 2A(-c_-\kappa\boldsymbol{m}_{2-}\sin(\kappa z) - c_+k\boldsymbol{m}_{2+}\sin(kz)) \\ &- (\hbar/e)\tau_{\mathrm{F}}\hat{\boldsymbol{y}} \times (ic_-\boldsymbol{m}_{2-}\omega\cos(\kappa z) + ic_+\boldsymbol{m}_{2+}\omega\cos(kz) - i\boldsymbol{m}_{1,0}\omega) \\ &+ (\hbar/e)\tau_{\mathrm{D}}(ic_-\boldsymbol{m}_{2-}\omega\cos(\kappa z) + ic_+\boldsymbol{m}_{2+}\omega\cos(kz) - i\boldsymbol{m}_{1,0}\omega) \\ &- J(-c_-\boldsymbol{m}_{2-}\cos(\kappa z) - c_+\boldsymbol{m}_{2+}\cos(kz) + \boldsymbol{m}_{1,0}) \end{aligned} \tag{S9.16}$$

where we have used $\hat{\boldsymbol{y}} \times (\hat{\boldsymbol{y}} \times \boldsymbol{m}_i) = -\boldsymbol{m}_i$ in the first step. In the second step we have used Eq. (S9.14), and the fact that the dynamic YIG magnetization must obey the boundary conditions for all times $t$. To solve for the coefficients $c_\pm$, we multiply the above equation with the complex conjugates of the YIG magnetization eigenvectors $\boldsymbol{m}_{2\pm}^*$, which obey the special orthogonality relations $\boldsymbol{m}_{2\mp}\boldsymbol{m}_{2\pm}^* = 0$. From the multiplication of $\boldsymbol{m}_{2+}^*$ we obtain:

$$\begin{aligned} 0 = \boldsymbol{m}_{2+}^*\big[& - 2Ac_+k\boldsymbol{m}_{2+}\sin(kz) \\ &- (\hbar/e)\tau_{\mathrm{F}}\hat{\boldsymbol{y}} \times (ic_-\boldsymbol{m}_{2-}\omega\cos(\kappa z) + ic_+\boldsymbol{m}_{2+}\omega\cos(kz) - i\boldsymbol{m}_{1,0}\omega) \\ &+ (\hbar/e)\tau_{\mathrm{D}}(ic_+\boldsymbol{m}_{2+}\omega\cos(kz) - i\boldsymbol{m}_{1,0}\omega) \\ &- J(-c_+\boldsymbol{m}_{2+}\cos(kz) + \boldsymbol{m}_{1,0})\big]. \end{aligned} \tag{S9.17}$$

From the multiplication of $\boldsymbol{m}_{2-}^{*}$ we obtain:

$$\begin{aligned}0 = \boldsymbol{m}_{2-}^{*}\big[&-2Ac_{-}\kappa\boldsymbol{m}_{2-}\sin(\kappa z)\\&-(\hbar/e)\tau_{\mathrm{F}}\hat{\boldsymbol{y}}\times(ic_{-}\boldsymbol{m}_{2-}\omega\cos(\kappa z)+ic_{+}\boldsymbol{m}_{2+}\omega\cos(kz)-i\boldsymbol{m}_{1,0}\omega)\\&+(\hbar/e)\tau_{\mathrm{D}}(ic_{-}\boldsymbol{m}_{2-}\omega\cos(\kappa z)-i\boldsymbol{m}_{1,0}\omega)\\&-J(-c_{-}\boldsymbol{m}_{2-}\cos(\kappa z)+\boldsymbol{m}_{1,0})\big].\end{aligned} \tag{S9.18}$$

We now can solve the system of equations consisting of Eq. (S9.17) and Eq. (S9.18) to obtain the complex coefficients $c_{\pm}$ as a function of the four variables $\boldsymbol{m}_1(\hat{\boldsymbol{y}}\times\boldsymbol{m}_{2\pm})$ and $\boldsymbol{m}_{2\mp}(\hat{\boldsymbol{y}}\times\boldsymbol{m}_{2\pm})$:

$$\begin{aligned}c_{\pm} = \frac{\pm 1}{c}\Bigg[&2A\kappa\sin(d\kappa)(J\boldsymbol{m}_{1,0}(\hat{\boldsymbol{y}}\times\boldsymbol{m}_{2\mp})-i(\hbar/e)\omega(\boldsymbol{m}_{1,0}\boldsymbol{m}_{2\mp}\tau_{\mathrm{F}}+\boldsymbol{m}_{1,0}(\hat{\boldsymbol{y}}\times\boldsymbol{m}_{2\mp})\tau_{\mathrm{D}}))\\&+\boldsymbol{m}_{1,0}(\hat{\boldsymbol{y}}\times\boldsymbol{m}_{2\mp})\cos(d\kappa)\left((\hbar/e)^2\omega^2\left(\tau_{\mathrm{D}}^2+\tau_{\mathrm{F}}^2\right)+2i(\hbar/e)J\tau_{\mathrm{D}}\omega-J^2\right)\Bigg]\end{aligned} \tag{S9.19}$$

where the prefactor $c$ is given by:

$$\begin{aligned}c = \cos(dk)\Bigg[&2A\kappa\sin(d\kappa)(J\boldsymbol{m}_{2+}(\hat{\boldsymbol{y}}\times\boldsymbol{m}_{2-})+i(\hbar/e)\omega(\boldsymbol{m}_{2-}(\hat{\boldsymbol{y}}\times\boldsymbol{m}_{2+})\tau_{\mathrm{D}}-\boldsymbol{m}_{2-}\boldsymbol{m}_{2+}\tau_{\mathrm{F}}))\\&+\boldsymbol{m}_{2+}(\hat{\boldsymbol{y}}\times\boldsymbol{m}_{2-})\cos(d\kappa)\left((\hbar/e)^2\omega^2\left(\tau_{\mathrm{D}}^2+\tau_{\mathrm{F}}^2\right)+2i(\hbar/e)J\tau_{\mathrm{D}}\omega-J^2\right)\Bigg]\\&+2Ak\sin(dk)\Bigg[-2A\kappa\boldsymbol{m}_{2+}(\hat{\boldsymbol{y}}\times\boldsymbol{m}_{2-})\sin(d\kappa)+\cos(d\kappa)(J\boldsymbol{m}_{2+}(\hat{\boldsymbol{y}}\times\boldsymbol{m}_{2-})\\&+i(\hbar/e)\omega(\boldsymbol{m}_{2-}\boldsymbol{m}_{2+}\tau_{\mathrm{F}}+\boldsymbol{m}_{2-}(\hat{\boldsymbol{y}}\times\boldsymbol{m}_{2+})\tau_{\mathrm{D}}))\Bigg].\end{aligned} \tag{S9.20}$$

The complex coefficients $c_{\pm}$ now specify the YIG solution and contain the influence of the Co layer. Using the eigenvectors Eq. (S9.11) and Eq. (S9.10) together with the wavevectors Eq. (S9.6) and Eq. (S9.7) and the complex coefficients Eq. (S9.20) and Eq. (S9.19) in the ansatz Eq. (S9.14) yields the spatially-dependent YIG magnetization. Using subsequently the ansatz Eq. (S9.14) and Eq. (S9.15) in the modified LLG Eq. (S9.2) allows to extract the Co susceptibility $\tilde{\boldsymbol{\chi}}_1$ by sorting the resulting expression by the transverse Co magnetization components $(m_{1,z}, m_{1,x})$. We find

$$\tilde{\boldsymbol{\chi}}_1^{-1} = \begin{pmatrix}\chi_{1,zz}^{-1} & \chi_{1,xz}^{-1}\\ \chi_{1,zx}^{-1} & \chi_{1,xx}^{-1}\end{pmatrix} \Longleftrightarrow \tilde{\boldsymbol{\chi}}_1 = \frac{1}{\chi_{1,zz}^{-1}\chi_{1,xx}^{-1}-\chi_{1,zx}^{-1}\chi_{1,xz}^{-1}}\begin{pmatrix}\chi_{1,xx}^{-1} & -\chi_{1,zx}^{-1}\\ -\chi_{1,xz}^{-1} & \chi_{1,zz}^{-1}\end{pmatrix} \tag{S9.21}$$

where the entries of the inverse susceptibility are:

$$\chi_{1,zz}^{-1} = \frac{i\alpha_1\omega}{\gamma_1}+\boldsymbol{m}_2(d_2)\frac{-i(\hbar/e)\tau_{\mathrm{D}}\omega+i(\hbar/e)\tau_{\mathrm{F}}\omega+J}{d_1M_{\mathrm{s},1}}+\frac{i(\hbar/e)\tau_{\mathrm{D}}\omega-J}{d_1M_{\mathrm{s},1}}-\mu_0(H+M_{\mathrm{s},1}), \tag{S9.22}$$

$$\chi_{1,zx}^{-1} = -\frac{i\omega}{\gamma_1}+\boldsymbol{m}_2(d_2)\frac{-i(\hbar/e)\tau_{\mathrm{D}}\omega+i(\hbar/e)\tau_{\mathrm{F}}\omega+J}{d_1M_{\mathrm{s},1}}-\frac{i(\hbar/e)\tau_{\mathrm{F}}\omega}{d_1M_{\mathrm{s},1}}, \tag{S9.23}$$

$$\chi_{1,xz}^{-1} = \frac{i\omega}{\gamma_1}+\boldsymbol{m}_2(d_2)\frac{-i(\hbar/e)\tau_{\mathrm{D}}\omega-i(\hbar/e)\tau_{\mathrm{F}}\omega+J}{d_1M_{\mathrm{s},1}}+\frac{i(\hbar/e)\tau_{\mathrm{F}}\omega}{d_1M_{\mathrm{s},1}}, \tag{S9.24}$$

$$\chi_{1,xx}^{-1} = \frac{i\alpha_1\omega}{\gamma_1}+\boldsymbol{m}_2(d_2)\frac{-i(\hbar/e)\tau_{\mathrm{D}}\omega-i(\hbar/e)\tau_{\mathrm{F}}\omega+J}{d_1M_{\mathrm{s},1}}+\frac{i(\hbar/e)\tau_{\mathrm{D}}\omega-J}{d_1M_{\mathrm{s},1}}-\mu_0H. \tag{S9.25}$$

However, an analytical solution of the resonance condition $\det\tilde{\boldsymbol{\chi}}_1^{-1} = 0$ is not possible. A numerical solution has been used to compute the results presented in the main text using

$$\chi_{1,xx} = \frac{\chi_{1,zz}^{-1}}{\chi_{1,zz}^{-1}\chi_{1,xx}^{-1}-\chi_{1,zx}^{-1}\chi_{1,xz}^{-1}}. \tag{S9.26}$$

Note that we can obtain analytical resonance conditions in the macrospin approximation. For this we have to

replace the spatially-dependent YIG magnetization by an uniform magnetization $\boldsymbol{m}_2(d_2) \to \boldsymbol{m}_2$ in Eq. (S9.2).

## S10. SIMULATION OF THE EXCHANGE MODE

Fig. S10 (a) shows the color map for a pure antiferromagnetic exchange coupling between the YIG and Co layers. We find an exchange mode at higher frequencies than the Co resonance and symmetric avoided crossings.

In Fig. S10 (b) we show the color map for a field-like torque which is substantially smaller than the damping-like torque. We observe a dominant mode-locking of the YIG and Co resonances. In metallic systems [20] we expect that the torques are primarily damping-like, as the real part of the spin mixing conductance exceeds the imaginary part. However, for insulating interfaces the amplitudes of the torques are less clear. Here, we find that our experiments are not reproduced with a dominant damping-like torque.

In Fig. S10 (c) we plot the color map for $\tau_\mathrm{F} = -30\ \mathrm{A\,s/m^2}$, $\tau_\mathrm{D} = 15\ \mathrm{A\,s/m^2}$ and $J = 0$. Note that this configuration refers to the situation of the YIG/Cu(5)/Co(50) sample from Fig. 1 (b),(e) with an inverted field-like torque. We find that the intensity symmetry of the avoided crossings is now also inverted compared to the experimental data (inset). Therefore, we know the sign of the field-like torque is positive for the YIG/Cu(5)/Co(50) samples.

In Fig. S10 (d) we show the color map for the YIG/Co(50) sample for a positive field-like torque and a strong antiferromagnetic coupling. The avoided crossings are symmetric, as the influence of the field-like torque is much smaller than the exchange torque. When we compare Fig. S6 (b), Fig. 3 (a), and Fig. S10 (d), we find that all used parameter combinations produce avoided crossings, with slightly different intensity modifications in the dispersion branches of the coupled systems. Due to the similar effects of the exchange torques and field-like torques, it is challenging to determine the signs of these torques for the YIG/Co samples without an interlayer.

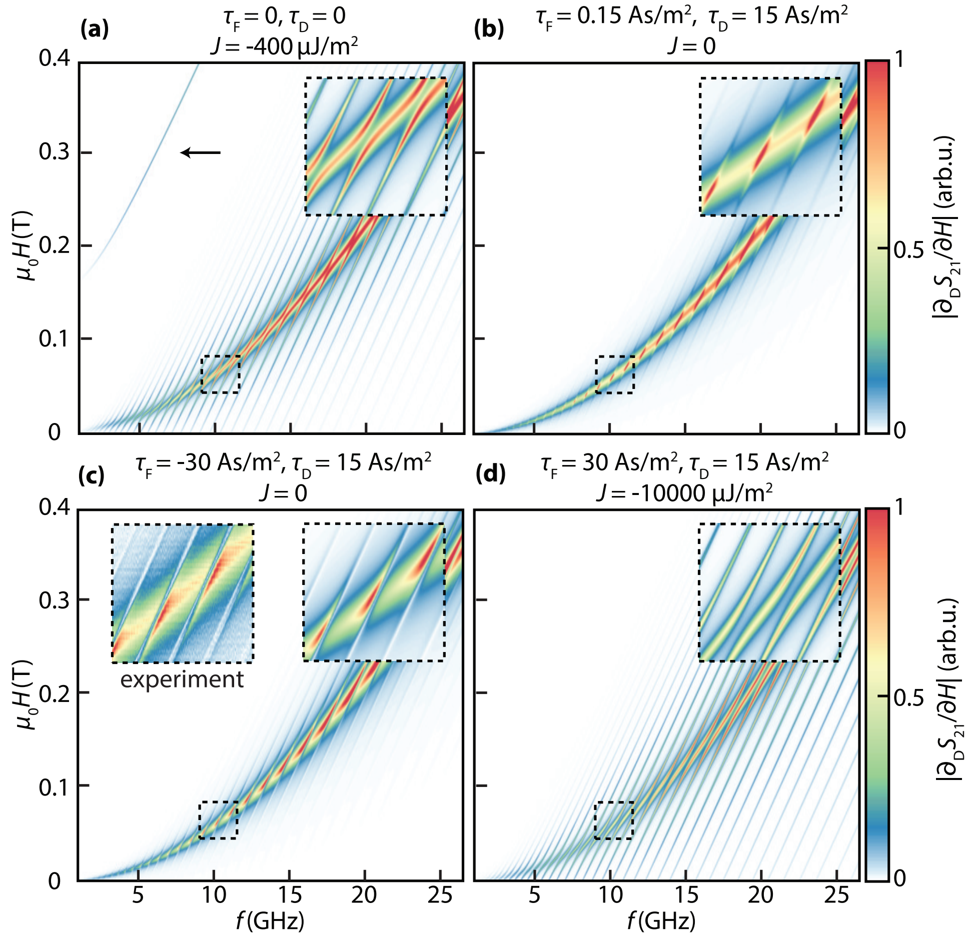


FIG. S10. (a) An exchange coupling can reproduce the exchange mode in the experiment. (b) A dominant damping-like torque results in a mode-locking of the YIG and Co resonances. (c) The sign of the field-like torques determines the asymmetry of the color code. We require a positive field-like torque to simulate the YIG/Cu(5)/Co(50) experiments, cf. Fig. 3 (b). (d) A dominant antiferromagnetic exchange torque produces symmetric avoided crossings.

[1] S. Pütter, S. Geprägs, R. Schlitz, M. Althammer, A. Erb, R. Gross, and S. T. B. Goennenwein, Applied Physics Letters **110**, 012403 (2017).

[2] H. Maier-Flaig, S. T. B. Goennenwein, R. Ohshima, M. Shiraishi, R. Gross, H. Huebl, and M. Weiler, (2017), arXiv:1705.05694.

[3] M. A. W. Schoen, J. M. Shaw, H. T. Nembach, M. Weiler, and T. J. Silva, Physical Review B **92**, 184417 (2015).

[4] A. J. Berger, E. R. J. Edwards, H. T. Nembach, J. M. Shaw, A. D. Karenowska, M. Weiler, and T. J. Silva, (2016), arXiv:1611.05798.

[5] S. Klingler, A. V. Chumak, T. Mewes, B. Khodadadi, C. Mewes, C. Dubs, O. Surzhenko, B. Hillebrands, and A. Conca, Journal of Physics D: Applied Physics **48**, 015001 (2015).

[6] C. Dubs, O. Surzhenko, R. Linke, A. Danilewsky, U. Brückner, and J. Dellith, Journal of Physics D: Applied Physics **50**, 204005 (2017).

[7] G. Carlotti, G. Gubbiotti, L. Pareti, G. Socino, and G. Turilli, Journal of Magnetism and Magnetic Materials **165**, 424 (1997).

[8] P. Hansen, P. Röschmann, and W. Tolksdorf, Journal of Applied Physics **45**, 2728 (1974).

[9] A. G. Gurevich and A. N. Anisimov, Sov Phys JETP **41**, 336 (1975).

[10] P. F. Herskind, A. Dantan, J. P. Marler, M. Albert, and M. Drewsen, Nature Physics **5**, 494 (2009).

[11] H. Maier-Flaig, M. Harder, R. Gross, H. Huebl, and S. T. B. Goennenwein, Physical Review B **94**, 054433 (2016).

[12] P. Landeros and D. L. Mills, Physical Review B **85**, 054424 (2012).

[13] M. Körner, K. Lenz, R. A. Gallardo, M. Fritzsche, A. Mücklich, S. Facsko, J. Lindner, P. Landeros, and J. Fassbender, Physical Review B **88**, 054405 (2013).

[14] M. Krawczyk, S. Mamica, M. Mruczkiewicz, J. W. Klos, S. Tacchi, M. Madami, G. Gubbiotti, G. Duerr, and D. Grundler, Journal of Physics D: Applied Physics **46**, 495003 (2013).

[15] R. A. Gallardo, A. Banholzer, K. Wagner, M. Körner, K. Lenz, M. Farle, J. Lindner, J. Fassbender, and P. Landeros, New Journal of Physics **16**, 023015 (2014).

[16] R. Arias and D. L. Mills, Physical Review B **60**, 7395 (1999).

[17] R. McMichael and P. Krivosik, IEEE Transactions on Magnetics **40**, 2 (2004).

[18] R. D. McMichael, Journal of Applied Physics **103** (2008), 10.1063/1.2837887.

[19] S. S. Kalarickal, P. Krivosik, M. Wu, C. E. Patton, M. L. Schneider, P. Kabos, T. J. Silva, and J. P. Nibarger, Journal of Applied Physics **99**, 093909 (2006).

[20] B. Heinrich, Y. Tserkovnyak, G. Woltersdorf, A. Brataas, R. Urban, and G. E. W. Bauer, Physical Review Letters **90**, 187601 (2003).
